# Supplementary material for: The Double-Edged Sword of Behavioral Responses in Strategic Classification: Theory and User Studies
Source: arXiv:2410.18066 source file (2024-10-25)
Supplement: Supplementary file 1 [file 11_Appendix_Warm_up.tex]

\section{Warm Up: One-dimensional features}
Consider the one-dimensional case where the classifier can be expressed as $h(x, \theta) = 1$ if and only if $x\ge \theta$, with $x, \theta \in [0,1]$. Assume we have a $\theta_0$, the non-strategic threshold, and a $\theta^*_\text{NB}$, the strategic threshold when the firm assumes agents are non-behavioral. From \citet{Milli2019socialcost} we already know $\theta_0 < \theta^*_\text{NB}$. However, if the agents are behavioral, this will not be the optimal threshold since the firm can increase its utility by considering agents' behavioral biases. To illustrate why this happens, consider the following setting; we know for behavioral agents and one-dimensional feature space, two scenarios can happen: (i) $w(\theta) < \theta$ and (ii) $w(\theta) > \theta$. Additionally, assume the firm does not know that the agents are behavioral, i.e., announces $\theta^*_\text{NB}$. 

\begin{proposition}\label{prop:B-NB_1D}
    For a one dimensional classifier, if $w(\theta)<\theta$, then $\theta^*_\text{B} = \theta_0 < \theta^*_\text{NB}$.
\end{proposition}
\begin{proof}
For this case, if $\tau^*_\text{NB}$ is announced, behavioral agents will react to $w(\tau^*_\text{NB})<\tau^*_\text{NB}$, so the agents that are manipulating their features will not be successful in their goal. They will only exert a \emph{behavioral cost} without being rewarded. Therefore, since the inequality is strict, there exists a $\tau^*_\text{B} < \tau^*_\text{NB}$ that lets the firm choose more qualified agents without worrying about accepting the unqualified agents that are gaming the features, which results in $\mathcal{U}(h(x, \tau^*_\text{B}))> \mathcal{U}(h(x, \tau^*_\text{NB}))$. Moreover, this case reduces to the case of non-responding agents, and the firm choosing $\tau_0$ will be optimal; the only difference would be the behavioral cost of unqualified agents, i.e., $c(x_\text{B}, x)$. 

Meaning that for $x<w(\tau^*_\text{B})$ we can write $\sP(h(\bar x_\text{B}, \theta)=y)=\sP(h(x, \theta)=y)$ because the total number of individuals below the threshold remain the same even though the distribution has changed. For $x>w(\tau^*_\text{B})$ nothing will be different since no one needs to manipulate their feature, and the distribution will also be the same as before, so we can write $\tau^*_\text{B}=\tau_0$.
\end{proof}

In Proposition~\ref{prop:B-NB_1D}, we see that by noticing the behavioral bias of the agents, the firm can increase their utility to the maximum. By defining \emph{individual burden} and \emph{social burden} as defined in \citet{Milli2019socialcost}, $b_h(x) = \min_{h(\hat x) = 1}c(\hat x, x)$ and $\mathcal{B}_{+}(h) = \mathbb{E}[b_h(x)|Y=1]$, respectively, and knowing that social burden is monotonically increasing in $\theta$, using Proposition~\ref{prop:B-NB_1D}, we can see from that for $w(\theta)<\theta$, the firm considering the behavioral bias of agents results in both increasing the utility of the firm and lowering the social burden, i.e., $\mathcal{U}
_\text{S}(h(x, \theta_{\text{B}})) > \mathcal{U}
_\text{S}(h(x, \theta_{\text{NB}}))$ and $\mathcal{B}
_{+}(\theta^*_\text{NB}) > \mathcal{B}
_{+}(\theta^*_\text{B}) = \mathcal{B}
_{+}(\theta_0)$ at the cost of lowering the utility of the agents manipulating their features by $c(\bar x_\text{B}, x)$. 

However, things will not be as smooth when $w(\theta)>\theta$ since the firm must find the tipping point according to the trade-off between accepting unqualified and not accepting qualified agents. 

\paragraph{A trade-off:} For the case where $w(\theta) > \theta$, if $\theta^*_\text{NB}$ is announced, the agents will react to $w(\theta^*_\text{NB}) 
> \theta^*_\text{NB}$ and the agents gaming their feature will not only successfully classify as qualified, but they will also be able to pass the threshold strictly. This means that the firm will be accepting unqualified individuals that have $x= w(\theta^*_\text{NB}) >\theta^*_\text{NB}$. Note that these agents will not surpass $x= w(\theta^*_\text{NB})$ since they will not receive any rewards, which will only be more costly. 

For $\theta > \theta^*_\text{NB}$, the firm will be cutting down the number of agents who choose to manipulate ($U_\text{B}>0$) at the cost of losing truly qualified agents. And, for $\theta < \theta^*_\text{NB}$, the firm will gain utility by accepting more qualified agents. Still, it will have a loss on utility by automatically accepting more unqualified agents, plus an additional loss by having agents manipulate their feature. 

Therefore, $\theta^*_\text{B}$ will be where the utility gained from not accepting the unqualified agents who manipulate equals the utility loss of not accepting the truly qualified agents. While discussing the decision boundary, agents' response, and firms' strategic choice in one dimension is simple, we miss a few crucial points compared to higher dimensions. In higher dimensions, we can have a subset of agents that (1) will manipulate their features not making it to the threshold while they could if they were not biased, (2) will manipulate their features and, despite being biased, will pass the threshold, (3) will not manipulate their features but they would if they were not biased, and (4) will manipulate their features even though they are positively classified! These subsets of agents are of interest as we can understand and respond to the collective behavior of users by anticipating and discussing these subsets. 
